# Supplementary material for: Given Enough Eyeballs, All Bugs Are Shallow? Revisiting Eric Raymond with Bug Bounty Programs
Source: arXiv:1608.03445 source file (2017-08-22)
Supplement: Supplementary file 1 [file appendix.tex]

\section*{Appendix}

\subsubsection{Derivations of the Model for homogenous factors $\Lambda_k = \Lambda$}
\label{derivation}
Here, we provide a detailed study of the possible behaviors of the model, also around the critical point $\Lambda =1$.

Three regimes must be considered:
\begin{enumerate}
\item For $\Lambda < 1$, the distribution is given by
\be
P_{\Lambda <1}(S  \geq s) = (1-\beta) \left(1 - {s \over s_{\rm max}}\right)^c~, ~~~s_{\rm max} := {S_0 \Lambda \over 1-\Lambda}~, ~~c := {\rm{ln}{\beta} 
\over \rm{ln}{\Lambda}} >0~.
\label{trjruyk5i}
\ee
This distribution can be approximated in its central part, away from the maximum possible reward $s_{\rm max}$,
by a Weibull distribution of the form

\be
{\rm Pr}_{\rm }({\rm S} \geq s) \sim e^{-(s/d)^{c}}~.
\label{trjeargquju}
\ee

For $\Lambda \to 1^-$, 
we have $s_{\rm max} \to +\infty$ and, for $s \ll s_{\rm max}$,
expression (\ref{trjruyk5i}) simplifies into a simple exponential function 
\be
P_{\Lambda \to 1^-}(S  \geq s) \sim e^{-|\ln(\beta)| s/S_0}~.
\label{jrtikik}
\ee

\item For $\Lambda = 1$, the distribution of rewards  is a simple exponential function since $S_{n} = n S_{0}$ is linear in the rank $n$ and the probability of reaching rank $n$ is the exponential
$P(n) = \beta^{n} (1-\beta)$. Actually, the expression
(\ref{jrtikik}) becomes asymptotical exact as
\be
P_{\Lambda =1}(S  \geq s) = (1-\beta) e^{-|\ln(\beta)| s/S_0}~.
\label{jrtikik}
\ee

\item For $\Lambda > 1$, the distribution of rewards is of the form,

\be
P_{\Lambda >1}(S  \geq s) = \frac{1}{{{(1+ \frac{s}{s*})}^{c}}}~,~~s^{*} := {S_0 \Lambda \over \Lambda -1}~, ~~c := {|\rm{ln}{\beta}|\over \rm{ln}{\Lambda}}~,
\label{jrtisdfjl}
\ee

which develops to a power law distribution of reward of the form
${\rm Pr}({\rm reward} \geq S) = C/S^{\mu}$ with $\mu = c$, when $\Lambda \rightarrow +\infty$.

%For $\Lambda \to 1^+$, the tail is still power law and the exponent $\mu$ grows without bound if the probability $\beta$ does not converge to $1$ at the same rate.  Denoting $\Lambda = 1-a$, $\beta = 1-\rho a$, with $a \to 0^+$ and $\rho$ constant, we have $\mu \to \rho$.
\end{enumerate}
